# Supplementary material for: GAQAT: gradient-adaptive quantization-aware training for domain generalization
Source: arXiv:2412.05551 source file (2024-12-07)
Supplement: Supplementary file 1 [file appendix.tex]

\appendix
\section{Appendix}
You may include other additional sections here.

% 可能得放实验结果 以及  扰动scale的情况
